# Supplementary material for: Simulating Errors in Touchscreen Typing
Source: arXiv:2502.03560 source file (2025-02-05)
Supplement: Supplementary file 1 [file Appendix.tex]

\section{Joint optimization of parameters}
\label{appendix:optimization}

To optimize \name, we used a two-loop process designed to find the best set of reward, model, and human parameters. This process aims to minimize the difference between the agent's predicted typing patterns and actual human typing patterns, ensuring realistic and effective interactions.

Both loops are guided by a Bayesian Optimization (BO) framework, chosen for its efficiency in handling high-dimensional objective functions. BO uses a probabilistic surrogate model to predict the performance of different parameter sets, reducing the number of evaluations required. This approach allows for an efficient search through the parameter space, resulting in a robust typing model that performs well across various scenarios.

The overall optimization algorithm is presented in Algorithm~\ref{alg:opt}.

\begin{algorithm}
    \caption{Joint Optimization of Parameters}\label{alg:opt}
    \begin{algorithmic}[1]
    \Require Define the search space of parameters to optimize.
    \newline $\mathcal{X}_{r}$: search space of reward parameters; 
    \newline$\mathcal{X}_{model}$: search space of model parameters; 
    \newline$\mathcal{X}_{human}$: search space of human parameters.
    % $f$ : objective function
    \While{\textit{outer loop}: optimal $r^*$ and $\boldsymbol{\theta}_{model}^*$ has not been found}
    \State Jointly select $r \in \mathcal{X}_{r}$ and $\theta_{model} \in \mathcal{X}_{model}$ using Bayesian optimization.
    \State Train model $\mathcal{M}(\theta_{model})$ with $r$, $\theta_{policy}$ and $\theta_{human} \in \mathcal{X}_{human}$ randomly sampled in each training episode.
    \While{\textit{inner loop}: optimal $\boldsymbol{\theta}_{human}^*$ has not been found}
    \State Select parameters $\theta_{human} \in \mathcal{X}_{human}$ via Bayesian optimization
    \State Sample $n$ typing episodes ($\boldsymbol{\tau}_1$, $\boldsymbol{\tau}_2$, ..., $\boldsymbol{\tau}_{n}$) from the model $\mathcal{M}(\boldsymbol{\theta}_{env};\boldsymbol{\theta}_{human})$
    \State Compute the metrics $Metrics(\boldsymbol{\tau}_1, \boldsymbol{\tau}_2, ..., \boldsymbol{\tau}_{n})$ 
    \State Evaluate with human data: $JS(Metrics(\boldsymbol{\tau}_1, \boldsymbol{\tau}_2, ..., \boldsymbol{\tau}_{n}), Metrics({h}_1, {h}_2, ..., {h}_{n}))$ 
    \EndWhile
    %\State Sample $n$ typing episodes ($\boldsymbol{\tau}_1$, $\boldsymbol{\tau}_2$, ..., $\boldsymbol{\tau}_{n}$) from the model $\mathcal{M}(\boldsymbol{\theta}_{env};\boldsymbol{\theta}^*_{human})$
    %\State Compute the metrics $Metrics(\boldsymbol{\tau}_1, \boldsymbol{\tau}_2, ..., \boldsymbol{\tau}_{n})$ 
    %\State Evaluate with human data: $JS(Metrics(\boldsymbol{\tau}_1, \boldsymbol{\tau}_2, ..., \boldsymbol{\tau}_{n}), Metrics({h}_1, {h}_2, ..., {h}_{n}))$ 
    \EndWhile
    \State \textbf{return}: general model $\mathcal{M}(\boldsymbol{\theta}^*_{model})$, and user-fitted parameters $\boldsymbol{\theta}^*_{human}$
    \end{algorithmic}
\end{algorithm}

\subsection{Outer Loop Optimization}
The outer loop focuses on optimizing parameters that influence both the reward system and the agent's training process. These parameters directly affect how the agent interacts with the environment and learns from these interactions. Key parameters optimized in this loop include:
    \begin{itemize}
        \item \textbf{Reward Parameters}: These parameters control how rewards are given to the RL agent based on typing accuracy and time efficiency. The reward $r$ is defined as:
        \begin{equation}
        \mathcal{R} = (1 - \text{Err}^{\alpha}) - w \cdot t,
        \end{equation}
        where:
        \begin{itemize}
            \item $\alpha$: exponential power constant that adjusts the sensitivity of the reward to the character error rate (cer).
            \item $w$: weight for time in the reward calculation.
            \item cer: character error rate, indicating the percentage of incorrectly typed characters.
            \item $t$: typing time.
        \end{itemize}
        The parameters $w$, and $\alpha$ are the ones optimized in the outer loop.
        \item \textbf{Training Parameters}: These parameters control various aspects of the agent's training process, such as exploration and learning from experiences:
        \begin{itemize}
            \item Lambda parameter for Generalized Advantage Estimation (GAE), which affects the trade-off between bias and variance in advantage estimation during training.
            \item Discount factor for future rewards, which determines how much the agent values immediate rewards compared to future rewards.
            \item Learning rate, which defines the step size for the optimization algorithm and affects how quickly or slowly the model learns from new data.
            \item Number of training epochs, which determines how many times the learning algorithm updates the model parameters per training iteration.
            \item Entropy coefficient, which encourages exploration by penalizing deterministic policies, helping the agent explore a wider range of actions.
            \item Clipping range for policy updates, which helps stabilize training by preventing large updates that could destabilize the policy.
        \end{itemize}
        \item \textbf{Neural Network Architecture Parameters}: These parameters define the architecture of the neural networks used by the RL agent, which affects its ability to learn and generalize from data. Specifically, the number of layers and the number of neurons in each layer of the policy network are optimized for the typing agent.
    \end{itemize}

\subsection{Inner Loop Optimization}
Within each iteration of the outer loop, the inner loop optimizes human parameters to adapt the agent to different user behaviors. These parameters capture variations in typing speed, accuracy, and style, and include:
    \begin{itemize}
        \item Memory retention: Reflects the user's ability to remember key placements and typing patterns.
        \item Finger dexterity: Represents the user's typing speed and finger movement efficiency.
        \item Vision acuity: Indicates the user's visual precision in locating keys.
        \item Proofreading errors: Accounts for mistakes made during the proofreading process.
        \item Guidance mistakes: Measures errors due to incorrect guidance or decision-making while typing.
        \item Forgetting rate: Captures the rate at which the user forgets key placements or typed content. 
        \item Bouncing rate: Represents the frequency of repeated key presses (e.g., double-pressing a key unintentionally).
        \item Order errors: Reflects the occurrence of typing characters in the wrong order.
    \end{itemize}
This inner loop ensures that the model is adaptable to individual user behaviors, enhancing its generalization capabilities.

% Both the outer and inner loops use a Bayesian Optimization (BO) framework to guide the search for optimal parameters. BO is useful for this problem because it efficiently handles high-dimensional and expensive objective functions. Manually searching for the optimal parameters would be impractical due to the large and complex parameter space, where interactions between parameters can have non-linear effects on the model's performance. BO addresses this challenge by using a probabilistic surrogate model to predict the performance of different parameter sets and strategically sampling from this model to find the optimum with fewer evaluations \cite{frazier_tutorial_2018}. This approach reduces the computational resources and time needed to identify high-performing parameters.

% \input{Tables/parameters}
